# Supplementary material for: AutoDirector: Online Auto-scheduling Agents for Multi-sensory Composition
Source: arXiv:2408.11564 source file (2024-08-21)
Supplement: Supplementary file 1 [file 0A_Appendix.tex]

\section*{Reproducibility Checklist}
This paper:
\begin{itemize}
\item Includes a conceptual outline and/or pseudocode description of AI methods introduced (yes)
\item Clearly delineates statements that are opinions, hypothesis, and speculation from objective facts and results (yes)
\item Provides well marked pedagogical references for less-familiare readers to gain background necessary to replicate the paper (yes)
\end{itemize}
Does this paper make theoretical contributions? (no)

If yes, please complete the list below.
\begin{itemize}
\item All assumptions and restrictions are stated clearly and formally. (NA)
\item All novel claims are stated formally (e.g., in theorem statements). (NA)
\item Proofs of all novel claims are included. (NA)
\item Proof sketches or intuitions are given for complex and/or novel results. (NA)
\item Appropriate citations to theoretical tools used are given. (NA)
\item All theoretical claims are demonstrated empirically to hold. (NA)
\item All experimental code used to eliminate or disprove claims is included. (NA)
\end{itemize}
Does this paper rely on one or more datasets? (no)

If yes, please complete the list below.
\begin{itemize}
\item A motivation is given for why the experiments are conducted on the selected datasets (NA)
\item All novel datasets introduced in this paper are included in a data appendix. (NA)
\item All novel datasets introduced in this paper will be made publicly available upon publication of the paper with a license that allows free usage for research purposes. (NA)
\item All datasets drawn from the existing literature (potentially including authors’ own previously published work) are accompanied by appropriate citations. (NA)
\item All datasets drawn from the existing literature (potentially including authors’ own previously published work) are publicly available. (NA)
\item All datasets that are not publicly available are described in detail, with explanation why publicly available alternatives are not scientifically satisficing. (NA)
\end{itemize}
Does this paper include computational experiments? (yes)

If yes, please complete the list below.
\begin{itemize}
\item Any code required for pre-processing data is included in the appendix. (yes).
\item All source code required for conducting and analyzing the experiments is included in a code appendix. (yes)
\item All source code required for conducting and analyzing the experiments will be made publicly available upon publication of the paper with a license that allows free usage for research purposes. (yes)
\item All source code implementing new methods have comments detailing the implementation, with references to the paper where each step comes from (yes)
\item If an algorithm depends on randomness, then the method used for setting seeds is described in a way sufficient to allow replication of results. (yes)
\item This paper specifies the computing infrastructure used for running experiments (hardware and software), including GPU/CPU models; amount of memory; operating system; names and versions of relevant software libraries and frameworks. (yes)
\item This paper formally describes evaluation metrics used and explains the motivation for choosing these metrics. (yes)
\item This paper states the number of algorithm runs used to compute each reported result. (yes)
\item Analysis of experiments goes beyond single-dimensional summaries of performance (e.g., average; median) to include measures of variation, confidence, or other distributional information. (yes)
\item The significance of any improvement or decrease in performance is judged using appropriate statistical tests (e.g., Wilcoxon signed-rank). (yes)
\item This paper lists all final (hyper-)parameters used for each model/algorithm in the paper’s experiments. (yes)
\item This paper states the number and range of values tried per (hyper-) parameter during development of the paper, along with the criterion used for selecting the final parameter setting. (yes)
\end{itemize}
